# Supplementary material for: Diffusion in mesoscopic lattice models of amorphous plasticity
Source: arXiv:1803.06009 ancillary file (2018-03-15)
Supplement: Supplementary file 1 [file TVM-SI.pdf]

# Supplementary Information to
# Diffusion in mesoscopic lattice models of amorphous plasticity

Botond Tyukodi,[1, 2, 3] Damien Vandembroucq,[1] and Craig E Maloney[2]

[1] *PMMH, ESPCI Paris/CNRS-UMR 7636/Univ. Paris 6 UPMC/Univ. Paris 7 Diderot/PSL Research Univ., 10 rue Vauquelin, 75231 Paris cedex 05, France*

[2] *Northeastern University, Department of Mechanical and Industrial Engineering Boston, USA*

[3] *Babeş - Bolyai University, Department of Physics Cluj-Napoca, Romania*

(Dated: March 15, 2018)

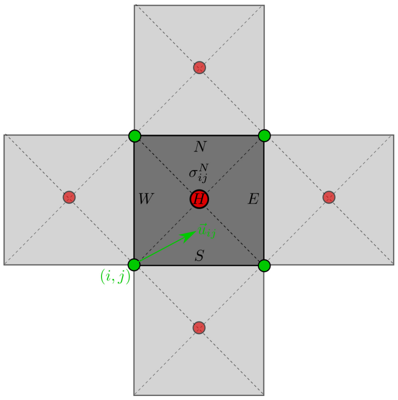


FIG. S1. Discretization of the elastic kernel: the plane is tiled by squares and each square is further divided into four sub-triangles.

## S1. DISCRETIZATION ON LATTICE OF THE ELASTIC RESPONSE TO A PLASTIC INCLUSION

As it has been pointed out in the main text, the system is particularly sensitive to the elastic kernel's discretization, therefore, unlike in most studies, here we provide full technical details regarding our discretization scheme. We note that our method is very similar to that of Nicolas et al [**?** ].

Our discretization is illustrated in Figure S1. The material is discretized on a square lattice. Displacements and forces are defined on the nodes of the grid, whereas stresses and strains are defined on the square plaquettes. In order to avoid checkerboard artefacts (as denoted in [**?** ]), we further subdivide each square plaquette into four sub-triangles. Each triangle is assigned a strain energy function and the strain energy of a plaquette is computed as the average strain energy over the four sub-triangles. It is assumed that each triangle has a homogeneous strain and the strain/stress on the square plaquette is then defined as the average of the strain/stress over the four triangles. It is further assumed that the middle node (i. e. the intersection of the four sub-triangles) slaves the corner nodes such that its displacement is given by the average of the four corner node displacements. This imposes an extra constraint and eliminates the degree of freedom associated to the middle node.

Although we introduce the sub-triangles, we end up working with square plaquettes since all quantities are averages over the sub-triangles. In particular, whenever a plastic event takes place, the whole plaquette (i. e. all its sub-triangles) yield. Similarly, the local thresholds are to be compared to the average stress on the plaquette.

### A. Node displacements to plaquette strains

Let us denote by $u^\alpha_{ij}$ the $\alpha$ cartesian component of the $ij$ node's displacement, by $u^\alpha_{Hij}$ the $\alpha$ cartesian component of the $ij$ middle node's displacement and by $a$ the lattice spacing. Then, for the left triangle's strain labeled as $W$ from "West" we have

$$u^\alpha_{Hij} - u^\alpha_{ij} = \frac{\partial u^\alpha_{ij}}{\partial x}\frac{a}{2} + \frac{\partial u^\alpha_{ij}}{\partial y}\frac{a}{2} = \epsilon^{\alpha x W}_{ij}\frac{a}{2} + \epsilon^{\alpha y W}_{ij}\frac{a}{2} \tag{S1}$$

$$u^\alpha_{Hij} - u^\alpha_{ij+1} = \frac{\partial u^\alpha_{ij}}{\partial x}\frac{a}{2} - \frac{\partial u^\alpha_{ij}}{\partial y}\frac{a}{2} = \epsilon^{\alpha x W}_{ij}\frac{a}{2} - \epsilon^{\alpha y W}_{ij}\frac{a}{2} \tag{S2}$$

which, solving for $\epsilon^{\alpha x W}_{ij}$, $\epsilon^{\alpha y W}_{ij}$ gives the strain as a function of node displacements in triangle $W$. Similar relations can be written for all the other triangles so finally we have

$$\epsilon^{\alpha x W}_{ij} = \frac{1}{a}[2u^\alpha_{Hij} - u^\alpha_{ij} - u^\alpha_{ij+1}] \qquad \epsilon^{\alpha y W}_{ij} = \frac{1}{a}[u^\alpha_{ij+1} - u^\alpha_{ij}] \tag{S3}$$

$$\epsilon^{\alpha x N}_{ij} = \frac{1}{a}[u^\alpha_{i+1j+1} - u^\alpha_{ij+1}] \qquad \epsilon^{\alpha y N}_{ij} = \frac{1}{a}[-2u^\alpha_{Hij} + u^\alpha_{ij+1} + u^\alpha_{i+1j+1}] \tag{S4}$$

$$\epsilon^{\alpha x E}_{ij} = \frac{1}{a}[-2u^\alpha_{Hij} + u^\alpha_{i+1j+1} + u^\alpha_{i+1j}] \qquad \epsilon^{\alpha y E}_{ij} = \frac{1}{a}[-u^\alpha_{i+1j} + u^\alpha_{i+1j+1}] \tag{S5}$$

$$\epsilon_{ij}^{\alpha xS} = \frac{1}{a}[-u_{ij}^{\alpha} + u_{i+1j}^{\alpha}] \quad \epsilon_{ij}^{\alpha yS} = \frac{1}{a}[2u_{Hij}^{\alpha} - u_{i+1j}^{\alpha} - u_{ij}^{\alpha}] \tag{S6}$$

The strain within plaquette $(i, j)$ is then given by the average over the 4 triangles:

$$\epsilon_{ij}^{\alpha\beta} = \frac{1}{4}[\epsilon_{ij}^{\alpha\beta N} + \epsilon_{ij}^{\alpha\beta E} + \epsilon_{ij}^{\alpha\beta S} + \epsilon_{ij}^{\alpha\beta W}] \tag{S7}$$

Note that terms containing middle node displacements $u_H$ are substituted with the corner nodes' average displacements:

$$u_{Hij}^{\alpha} = \frac{1}{4}[u_{ij}^{\alpha} + u_{i+1j}^{\alpha} + u_{i+1j+1}^{\alpha} + u_{ij+1}^{\alpha}] \tag{S8}$$

### B. Plaquette strains to forces

In this scheme, we associate a strain energy density to each of the triangles. The strain energy density on the square plaquette is then the average strain energy density over the trianles. The strain energy is quadratic in strains, as follows:

$$\Phi_{ijt} = \frac{K}{2}e_{1ijt}^2 + \frac{\mu}{2}e_{2ijt}^2 + \frac{\mu}{2}e_{3ijt}^2 \quad \text{for } t \ \in \{N, S, E, W\} \tag{S9}$$

where $K$ is the bulk modulus and $\mu$ is the shear modulus of the material, and the three deformation modes are $e_{1ij} = (1/2)(\epsilon_{ij}^{xx} + \epsilon_{ij}^{yy})$, $e_{2ij} = (1/2)(\epsilon_{ij}^{xx} - \epsilon_{ij}^{yy})$, $e_{3ij} = (1/2)(\epsilon_{ij}^{xy} + \epsilon_{ij}^{yx})$. The energy density of the plaquette is the average of the four triangles:

$$\Phi_{ij} = \frac{1}{4}\left(\Phi_{ijN} + \Phi_{ijS} + \Phi_{ijE} + \Phi_{ijW}\right) \tag{S10}$$

The total energy of the system is $\Phi = \sum_{ij} \Phi_{ij}$ and the force acting on node $(i, j)$ is given by the potential energy gradient $F_{ij} = -\nabla_{ij}\Phi$:

$$F_{ij}^{\alpha} = -\frac{\partial \Phi}{\partial u_{ij}^{\alpha}} = -\left(\frac{\partial \Phi_{i-1j-1}}{\partial u_{ij}^{\alpha}} + \frac{\partial \Phi_{ij-1}}{\partial u_{ij}^{\alpha}} + \frac{\partial \Phi_{i-1j}}{\partial u_{ij}^{\alpha}} + \frac{\partial \Phi_{ij}}{\partial u_{ij}^{\alpha}}\right), \quad \text{for } \alpha \in \{x, y\} \tag{S11}$$

All the other derivatives are zero since the energy of a plaquette only depends on the displacements on its nodes.

In the presence of external forces, the equilibrium equations are:

$$F_{ij}^{\alpha} + F_{ext\ ij}^{\alpha} = 0 \tag{S12}$$

which are nothing but the discrete form of the Lame-Navier equation. Since the elastic forces are linear in displacements:

$$F_{ij}^{\alpha} = \sum_{pq\beta} \frac{\partial F_{ij}^{\alpha}}{\partial u_{pq}^{\beta}} u_{pq}^{\beta} = -\sum_{pq\beta} \frac{\partial^2 \Phi}{\partial u_{ij}^{\alpha} \partial u_{pq}^{\beta}} u_{pq}^{\beta} = -\sum_{pq\beta} H_{ijpq}^{\alpha\beta} u_{pq}^{\beta} \tag{S13}$$

and the equilibrium equations can be rewritten as:

$$\sum_{pq\beta} H_{ijpq}^{\alpha\beta} u_{pq}^{\beta} = F_{ext\ ij}^{\alpha} \tag{S14}$$

### C. Building up the Hessian

When imposing periodic boundary conditions, the Hessian $H$ is translation invariant and it is possible to define the little Hessian $h$ such that:

$$h_{\Delta i\ \Delta j}^{\alpha\beta} = h_{p-i\ q-j}^{\alpha\beta} = H_{ijpq}^{\alpha\beta} \tag{S15}$$

and rewrite the equilibrium equations as:

$$\sum_{\beta \Delta i \Delta j} h^{\alpha\beta}_{\Delta i\ \Delta j} u^{\beta}_{i+\Delta i\ j+\Delta j} = F^{\alpha}_{ext\ ij} \tag{S16}$$

Evaluating the energy derivatives, one obtains for the elements of the little Hessian $h$:

$$h^{xx}_{-1,-1} = h^{xx}_{-1,1} = h^{xx}_{1,-1} = h^{xx}_{1,1} = \frac{1}{a^2}(-\mu - K/2) \tag{S17}$$

$$h^{xx}_{-1,0} = h^{xx}_{1,0} = \frac{1}{a^2}(-2\mu - 3K) \tag{S18}$$

$$h^{xx}_{0,-1} = h^{xx}_{0,1} = \frac{1}{a^2}(-2\mu + K) \tag{S19}$$

$$h^{xx}_{0,0} = \frac{1}{a^2}(12\mu + 6K) \tag{S20}$$

$$h^{xy}_{-1,-1} = h^{xy}_{1,1} = \frac{1}{a^2}(-K) \tag{S21}$$

$$h^{xy}_{-1,1} = h^{xy}_{1,-1} = \frac{1}{a^2}(K) \tag{S22}$$

$$h^{yy}_{-1,-1} = h^{yy}_{-1,1} = h^{yy}_{1,-1} = h^{yy}_{1,1} = \frac{1}{a^2}(-\mu - K/2) \tag{S23}$$

$$h^{yy}_{-1,0} = h^{yy}_{1,0} = \frac{1}{a^2}(-2\mu + K) \tag{S24}$$

$$h^{yy}_{0,-1} = h^{yy}_{0,1} = \frac{1}{a^2}(-2\mu - 3K) \tag{S25}$$

$$h^{yy}_{0,0} = \frac{1}{a^2}(12\mu + 6K) \tag{S26}$$

Note that $h^{xy}_{ij} = h^{yx}_{ij}$ and $h^{\alpha\beta}_{ij} = 0$ everywhere else.

### D. Solving the equilibrium equations

Upon imposed external forces therefore one has to invert the $H$ matrix in order to find the corresponding equilibrium displacement field. This can be accomplished exploiting the fact that $H$ is translation invariant, hence it commutes with the translation operator. Consequently, the eigenmodes of $H$ are the Fourier modes and its eigenvalues are given by the Fourier transform.

For better readability, we will use the braket notation for vectors and projections. $\hat{H}$ is a linear operator that, when feeded with the displacement field, returns the elastic force field:

$$\hat{H} \left| u \right\rangle = \left| F_{ext} \right\rangle \tag{S27}$$

We are, however, interested in its inverse in order to compute the displacement field for a given force field. Denoting by $\lambda_i$ the $i$-th eigenvalue and $|v^i\rangle = \{v^{i\alpha}_{mn}\}$ the $i$-th eigenvector of $\hat{H}$:

$$\hat{H} \left| v_i \right\rangle = \lambda_i \left| v_i \right\rangle \tag{S28}$$

$$\left\langle v_i \right| \hat{H} \left| u \right\rangle = \left\langle v_i | F_{ext} \right\rangle \tag{S29}$$

$$\lambda_i \left\langle v_i | u \right\rangle = \left\langle v_i | F_{ext} \right\rangle \Rightarrow \left\langle v_i | u \right\rangle = \frac{1}{\lambda_i} \left\langle v_i | F_{ext} \right\rangle \tag{S30}$$

The problem thus reduces to finding the eigenvalues and eigenvectors of $\hat{H}$.

Introducing the coordinate basis $|n^{lm\alpha}\rangle = \{\delta_{li}\delta_{mj}\delta_{\alpha\beta}\}$, for any vector $|u\rangle$ we have:

$$\left\langle n^{lm\alpha} | u \right\rangle = u^{\alpha}_{lm} \tag{S31}$$

and the $\hat{H}$ matrix elements are simply:

$$\left\langle n^{rs\beta} \right| \hat{H} \left| n^{lm\alpha} \right\rangle = \sum_{ijpq\delta\gamma} H^{\gamma\delta}_{ijpq} \delta_{pl}\delta_{qm}\delta_{\alpha\gamma}\delta_{ir}\delta_{js}\delta_{\delta\beta} = H^{\alpha\beta}_{rslm} = h^{\alpha\beta}_{r-l,s-m} \tag{S32}$$

Projecting eq. S28 to $\langle n^{lm\alpha}|$:

$$\langle n^{lm\alpha}|\,\hat{H}\,|v^i\rangle = \langle n^{lm\alpha}|\,\hat{H}\sum_{rs\beta}|n^{rs\beta}\rangle\,\langle n^{rs\beta}|v^i\rangle \tag{S33}$$

$$= \sum_{rs\beta}\langle n^{lm\alpha}|\,\hat{H}\,|n^{rs\beta}\rangle\,\langle n^{rs\beta}|v^i\rangle \tag{S34}$$

$$= \sum_{rs\beta} H^{\alpha\beta}_{lmrs}\,\langle n^{rs\beta}|v^i\rangle = \sum_{rs\beta} h^{\alpha\beta}_{r-l,s-m}\,\langle n^{rs\beta}|v^i\rangle \tag{S35}$$

$$= \lambda_i\,\langle n^{lm\alpha}|v^i\rangle \tag{S36}$$

Since $\hat{H}$ is translation invariant, it commutes with the translation operator $\hat{T}$ which means they must have a common eigenvector system. In $2D$, the eigenvectors of $\hat{T}$ are plane waves and have the form:

$$\langle n^{lm\alpha}|v^i\rangle = \frac{1}{NM}P^{pq}_{\alpha}\exp\left[2\pi i\left(\frac{lp}{N}+\frac{mq}{M}\right)\right] \tag{S37}$$

therefore it is reasonable to check the same form for the eigenvectors of $\hat{H}$. Plugging in S37 in the last equation of S36:

$$\sum_{rs\beta} h^{\alpha\beta}_{r-l,s-m}P^{pq}_{\beta}\exp[2\pi i\left(\frac{rp}{N}+\frac{sq}{M}\right)] = \lambda_i P^{pq}_{\alpha}\exp[2\pi i\left(\frac{lp}{N}+\frac{mq}{M}\right)] \tag{S38}$$

which leads to:

$$\sum_{\beta}\widetilde{h}^{\alpha\beta}_{pq}P^{pq}_{\beta} = \lambda_i P^{pq}_{\alpha} \tag{S39}$$

with $\alpha,\beta\in\{x,y\}$. Since $h^{\alpha\beta}_{lm}$ is sparse, its Fourier transform is easily computable:

$$\widetilde{h}^{xx}_{pq} = \frac{2}{a^2}\left[-(2\mu+3K)C_p + (-2\mu+K)C_q - (2\mu+K)(C_pC_q-3)\right] \tag{S40}$$

$$\widetilde{h}^{xy}_{pq} = \frac{4}{a^2}KS_pS_q \tag{S41}$$

$$\widetilde{h}^{yy}_{pq} = \frac{2}{a^2}\left[(-2\mu+K)C_p + (2\mu+3K)C_q - (2\mu+K)(C_pC_q-3)\right] \tag{S42}$$

$$\tag{S43}$$

with $C_p=\cos(2\pi p/N)$, $C_q=\cos(2\pi q/M)$, $S_p=\sin(2\pi p/N)$, $S_q=\sin(2\pi q/M)$. At this stage thus our problem has been reduced to finding the eigenvalues and eigenvectors of the $2\times 2$ matrix $\widetilde{h}^{\alpha\beta}_{pq}$. The resulting eigenvalues can be labeled as $\lambda_i\equiv\lambda^{\delta}_{pq}$ and their expression is:

$$\lambda^{x}_{pq} = \frac{2}{a^2}\left[(6\mu+5K) - (2\mu+K)(C_p+C_q) - (2\mu+3K)C_pC_q\right] \tag{S44}$$

$$\lambda^{y}_{pq} = \frac{2}{a^2}\left[(6\mu+K) - (2\mu+K)(C_p+C_q) - (2\mu-K)C_pC_q\right] \tag{S45}$$

while the corresponding eigenvectors $P^{pq}_{\alpha}\equiv P^{pq\delta}_{\alpha}$:

$$(P^{pqx}_{x},P^{pqx}_{y}) = \frac{1}{\sqrt{1+\tan^2\frac{\pi p}{N}\cot^2\frac{\pi q}{M}}}\left(\tan\frac{\pi p}{N}\cot\frac{\pi q}{M},\ 1\right) \tag{S46}$$

$$(P^{pqy}_{x},P^{pqy}_{y}) = \frac{1}{\sqrt{1+\cot^2\frac{\pi p}{N}\tan^2\frac{\pi q}{M}}}\left(-\cot\frac{\pi p}{N}\tan\frac{\pi q}{M},\ 1\right) \tag{S47}$$

The eigenvectors of $\hat{H}$ are then labeled as $|v^i\rangle\equiv|v^{pq\delta}\rangle$ and given by eq. S37.

### E. Point force on a node

As an intermediate problem, let us consider the displacement field generated by a point force acting on node $(i, j)$ along direction $\beta$. This force has the following form in the coordinate basis:

$$\langle n^{lm\alpha}|F\rangle = f_0\ \delta_{li}\delta_{mj}\delta_{\alpha\beta} \tag{S48}$$

The same force in the eigenbasis has the form:

$$\langle v^{pq\delta}|F\rangle = \sum_{lm\alpha} \langle v^{pq\delta}|n^{lm\alpha}\rangle \langle n^{lm\alpha}|F\rangle = f_0 \sum_{lm\alpha} \langle v^{pq\delta}|n^{lm\alpha}\rangle \delta_{li}\delta_{mj}\delta_{\alpha\beta} \tag{S49}$$

$$= f_0 \langle v^{pq\delta}|n^{ij\beta}\rangle = f_0 \langle n^{ij\beta}|v^{pq\delta}\rangle^* = f_0 P_\beta^{pq\delta} \exp\left[-2\pi i \left(\frac{ip}{N} + \frac{jq}{M}\right)\right] \tag{S50}$$

which immediately gives the solution for the displacement in the eigenbasis:

$$\langle v^{pq\delta}|u\rangle = \frac{1}{\lambda_{pq}^\delta} \langle v^{pq\delta}|F\rangle = \frac{1}{\lambda_{pq}^\delta} f_0 P_\beta^{pq\delta} \exp\left[-2\pi i \left(\frac{ip}{N} + \frac{jq}{M}\right)\right] \tag{S51}$$

Switching back to the coordinate basis, we finally obtain the displacement field:

$$u_{lm}^\alpha = \langle n^{lm\alpha}|u\rangle = \sum_{pq\delta} \langle n^{lm\alpha}|v^{pq\delta}\rangle \langle v^{pq\delta}|u\rangle \tag{S52}$$

$$= f_0 \sum_{pq\delta} \frac{P_\alpha^{pq\delta} P_\beta^{pq\delta}}{\lambda_{pq}^\delta} \exp\left[2\pi i \left(\frac{(l-i)p}{N} + \frac{(m-j)q}{M}\right)\right] \tag{S53}$$

$$= f_0 \sum_{pq} B_{pq}^{\alpha\beta} \exp\left[2\pi i \left(\frac{(l-i)p}{N} + \frac{(m-j)q}{M}\right)\right] \tag{S54}$$

where

$$B_{pq}^{\alpha\beta} = \sum_\delta \frac{P_\alpha^{pq\delta} P_\beta^{pq\delta}}{\lambda_{pq}^\delta} \tag{S55}$$

For a point force at the origin $(i, j) = (0, 0)$ the displacement is then given by a simple inverse discrete Fourier transform of the respective $B_{pq}^{\alpha\beta}$ components:

$$u_{lm}^\alpha = f_0 \sum_{pq} B_{pq}^{\alpha\beta} \exp\left[2\pi i \left(\frac{lp}{N} + \frac{mq}{M}\right)\right] \tag{S56}$$

$$\widetilde{u}_{pq}^\alpha = f_0 B_{pq}^{\alpha\beta} \tag{S57}$$

### F. Eigenstrain on a plaquette

When a plaquette undergoes a plastic deformation, its free energy changes. Let us suppose that plaquette $(l, m)$ suffers a plastic deformation along deformation mode 2, i.e. all its triangles undergoes the same amount of plastic strain. Then the energy density of the triangles becomes

$$\Phi_{ijt} = \frac{K}{2} e_{1ijt}^2 + \frac{\mu}{2}(e_{2ijt} - e_0\delta_{il}\delta_{lm})^2 + \frac{\mu}{2} e_{3ijt}^2 \quad \text{for } t\ \in \{N, S, E, W\} \tag{S58}$$

whereas the energy density of the plaquette is again the average over the four triangles: $\Phi_{ij} = \langle\Phi_{ijt}\rangle_{\{t\}}$. This change in the reference configuration of the plaquettes (i. e. introducing a plastic strain field $\epsilon_{0pq}$) changes the node forces:

$$F_{ij}^\alpha = \sum_{pq\beta} \frac{\partial F_{ij}^\alpha}{\partial u_{pq}^\beta} u_{pq}^\beta + \sum_{pq} \frac{\partial F_{ij}^\alpha}{\partial e_{0pq}} e_{0pq} = -\sum_{pq\beta} \frac{\partial^2 \Phi}{\partial u_{ij}^\alpha \partial u_{pq}^\beta} u_{pq}^\beta - \sum_{pq} \frac{\partial^2 \Phi}{\partial u_{ij}^\alpha \partial e_{0pq}} e_{0pq} \tag{S59}$$

$$= -\sum_{pq\beta} H_{ijpq}^{\alpha\beta} u_{pq}^\beta - F_{0ij}^\alpha \tag{S60}$$

where

$$F^{\alpha}_{0ij} = \sum_{pq} \frac{\partial^2 \Phi}{\partial u^{\alpha}_{ij} \partial e_{0pq}} e_{0pq} \tag{S61}$$

We then have inhomogeneous terms in the equilibrium equations:

$$\sum_{pq\beta} H^{\alpha\beta}_{ijpq} u^{\beta}_{pq} = F^{\alpha}_{ext\ ij} - F^{\alpha}_{0ij} \tag{S62}$$

meaning that eigenstrains have the same effect as an extra external force field. With an eigenstrain on a single plaquette $e_{0pq} = e_0 \delta_{lp} \delta_{mq}$ this additional force reads as

$$F^{\alpha}_{0ij} = \frac{\partial^2 \Phi}{\partial u^{\alpha}_{ij} \partial e_0} e_0 = e_0 \frac{\partial}{\partial e_0} \left[ \frac{\partial \Phi_{i-1j-1}}{\partial u^{\alpha}_{ij}} + \frac{\partial \Phi_{ij-1}}{\partial u^{\alpha}_{ij}} + \frac{\partial \Phi_{i-1j}}{\partial u^{\alpha}_{ij}} + \frac{\partial \Phi_{ij}}{\partial u^{\alpha}_{ij}} \right] \tag{S63}$$

Evaluating the derivatives:

$$F^{x}_{0\ l+1,m+1} = F^{x}_{0\ l+1,m} = F^{y}_{0\ l+1,m} = F^{y}_{0\ l,m} = \frac{2\mu}{a} e_0 \tag{S64}$$

$$F^{x}_{0\ l,m+1} = F^{x}_{0\ l,m} = F^{y}_{0\ l+1,m+1} = F^{y}_{0\ l,m+1} = -\frac{2\mu}{a} e_0 \tag{S65}$$

which proves that as far as the displacements are concerned, if plaquette $(l, m)$ undergoes an eigenstrain of magnitude $e_0$ along the $e_2$ mode, this is equivalent to applying a suitable quadrupole of forces to the vertices of that plaquette. Note that this is merely a recovery of the classical result of the Eshelby inclusions. A similar argument can be carried out for plastic strains along mode $e_3$.

The problem thus has reduced to the application of a force quadrupole to the four nodes of a tile. By superimposing the fields resulting from the four point forces, one finds the fields induced by a plastic strain.

## G. Computing the stress response

We have seen how to connect nodal displacements to plaquette strains. From strains it is fairly straightforward to obtain the stresses on the triangles for the three modes $M \in \{1, 2, 3\}$ via $\sigma^{M}_{ijt} = \partial\Phi/\partial e^{M}_{ijt}$. The stress on the plaquette is then the average over its component triangles. We have also seen that an eigenstrain on a plaquette is equivalent to a quadrupole of forces acting on the corners of that plaquette. Adding up the contributions of the four forces of the quadrupole, we obtain the following expressions for the stress components Fourier transform:

### *1. Eigenstrain along mode 2*

$$\begin{aligned}
\widetilde{\sigma}^{(1)}_{pq} &= -8K\mu e_0 \frac{C_q - C_p}{(6\mu + 5K) - (2\mu + K)(C_p + C_q) - (2\mu + 3K)C_p C_q} \\
\widetilde{\sigma}^{(2)}_{pq} &= \mu e_0 [\frac{4\mu}{1 - C_p C_q} (\frac{(C_p - C_q)^2}{(6\mu + 5K) - (2\mu + K)(C_p + C_q) - (2\mu + 3K)C_p C_q} \\
&+ \frac{S_p^2 S_q^2}{(6\mu + K) - (2\mu + K)(C_p + C_q) - (2\mu - K)C_p C_q}) - 1] \\
\widetilde{\sigma}^{(3)}_{pq} &= 4\mu^2 e_0 \frac{S_p S_q (C_p - C_q)}{1 - C_p C_q} [\frac{1}{(6\mu + 5K) - (2\mu + K)(C_p + C_q) - (2\mu + 3K)C_p C_q} \\
&- \frac{1}{(6\mu + K) - (2\mu + K)(C_p + C_q) - (2\mu - K)C_p C_q}]
\end{aligned} \tag{S66}$$

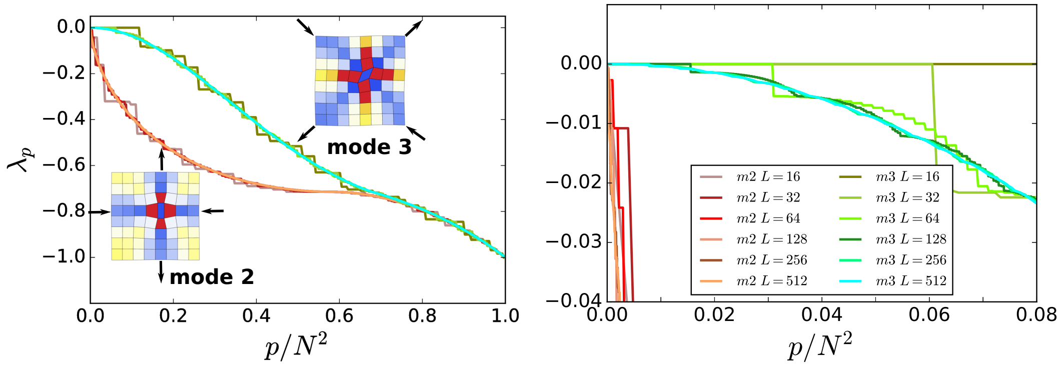


FIG. S2. Left, inset: discretized Eshelby kernel, $K^e(\mathbf{r}-\mathbf{r}')$, for mode 2 and mode 3 loading respectively for a lattice of size $L=8$. Left, main: Eigenvalues, $\lambda$, of the convolution operator as a function of mode index, $p$, for various $L$ for both mode 2 (red curves) and mode 3 (green curves). Right: Blow-up of the spectrum near $\lambda=0$.

### 2. *Eigenstrain along mode 3*

$$\widetilde{\sigma}_{pq}^{(1)} = 8K\mu e_0 \frac{S_p S_q}{(6\mu+5K)-(2\mu+K)(C_p+C_q)-(2\mu+3K)C_pC_q} \tag{S67}$$

$$\begin{aligned}\widetilde{\sigma}_{pq}^{(2)} &= 4\mu^2 e_0 \frac{S_pS_q(C_p-C_q)}{1-C_pC_q}\Big[\frac{1}{(6\mu+5K)-(2\mu+K)(C_p+C_q)-(2\mu+3K)C_pC_q} \\ &- \frac{1}{(6\mu+K)-(2\mu+K)(C_p+C_q)-(2\mu-K)C_pC_q}\Big]\end{aligned} \tag{S68}$$

$$\begin{aligned}\widetilde{\sigma}_{pq}^{(3)} &= \mu e_0\Big[\frac{4\mu}{1-C_pC_q}\Big(\frac{S_p^2S_q^2}{(6\mu+5K)-(2\mu+K)(C_p+C_q)-(2\mu+3K)C_pC_q} \\ &+ \frac{(C_p-C_q)^2}{(6\mu+K)-(2\mu+K)(C_p+C_q)-(2\mu-K)C_pC_q}\Big)-1\Big]\end{aligned}$$

### 3. *Soft deformation modes*

In Fig. S2, we show the Eshelby kernel in real space for mode 2 and 3 respectively. In Figs. S2c and S2d we plot the eigenvalue spectrum of the convolution operator for both loading modes for several $L$. Null modes of the convolution operator are present in mode 3. These correspond to perfect horizontal or vertical slip lines which completely span the system and result in no residual stress. No such null modes are possible in mode 2. The lowest $\lambda$ modes in mode 2 correspond to slip lines along the diagonal directions which unavoidably result in residual stress. However, we note that the minimum $\lambda$ for mode 2 goes to zero in the limit of $L\to\infty$ as shown on S3.

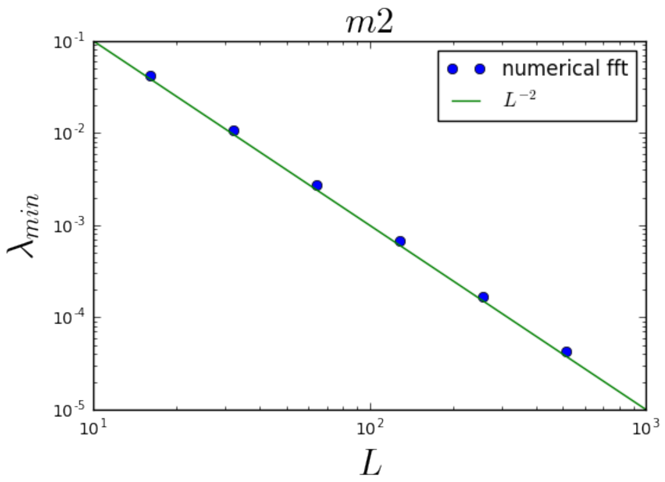


FIG. S3. System-size dependence of the smallest eigenvalue of the mode 2 kernel. As the system size increases, the eigenvalue approaches zero.
